# Supplementary material for: The Wreaths of KHAN: Uniform Graph Feature Selection with False Discovery Rate Control
Source: arXiv:2403.12284 source file (2024-03-18)
Supplement: Supplementary file 1 [file appendix.tex]

% !TEX root = main.tex

\newpage
